# Supplementary material for: Training Spiking Neural Networks Using Lessons From Deep Learning
Source: arXiv:2109.12894 source file (2023-08-13)
Supplement: Supplementary file 1 [file math.tex]

% figure B3
\documentclass{article}
\usepackage{amsmath}
\begin{document}
  \begin{align}
    y &= \begin{bmatrix}
           8 \\
           4 \\
           0
         \end{bmatrix}
  \end{align}

%   \rightarrow \vec{y}=1
  \begin{align}
    \begin{bmatrix}
           1 \\
           2 \\
           3
         \end{bmatrix}
  \end{align}

  \begin{equation}\label{beq:6}
    ,\hat{y} = 1
\end{equation}

%%%%%%%%%% figure b4
  \begin{align}
    \vec{y} &= \begin{bmatrix}
           1 \\
           0 \\
           0
         \end{bmatrix}
  \end{align}

%%%%%%%%%% figure b5

\begin{align}
    \vec{y} &= \begin{bmatrix}
           6 \\
           2 \\
           2
         \end{bmatrix}
  \end{align}

%%%%%%%%% figure b6
\begin{align}
    \vec{U}[t] &= \begin{bmatrix}
           U_1[t] \\
           U_2[t] \\
           U_3[t]
         \end{bmatrix}
  \end{align}

%%%%%% fig b8
Fig. b8: MS Spike Time
\begin{align}
    \vec{y}_1 &= \begin{bmatrix}
           0, 2, 5
         \end{bmatrix}
  \end{align}
  
  \begin{align}
    y_2 &= \begin{bmatrix}
           3
         \end{bmatrix}
  \end{align}
  
  \begin{align}
  y_3 &= \begin{bmatrix}
           5
         \end{bmatrix}
  \end{align}

%%%%%%%% fig b8
fig. b9 MS Membrane

\begin{align}
    y_1 &= \begin{bmatrix}
           \theta
         \end{bmatrix}
  \end{align}
  
  \begin{align}
    y_2 &= \begin{bmatrix}
           0
         \end{bmatrix}
  \end{align}
  
  \begin{align}
  y_3 &= \begin{bmatrix}
           0
         \end{bmatrix}
  \end{align}

\end{document}
